# Supplementary material for: Logical Majorana zero modes in a nanowire network
Source: arXiv:2210.07997 source file (2022-10-14)
Supplement: Supplementary file 1 [file appendix.tex]

\section{Counting neigboring sites of the wire network on which
  zero-mode in one site spills to}
\label{sec:appendix}
